# Supplementary material for: State-specific density functionals for excited states from ensembles
Source: arXiv:2406.18105 ancillary file (2024-10-14)
Supplement: Supplementary file 1 [file SuppMatt.v7.pdf]

# Supplementary Material for
# “Excitation energies from state-specific ensemble density functionals with density-driven correlations”

Tim Gould*

*Qld Micro- and Nanotechnology Centre,*
*Griffith University, Nathan, Qld 4111, Australia*

Stephen G. Dale

*Qld Micro- and Nanotechnology Centre,*
*Griffith University, Nathan, Qld 4111, Australia and*
*Institute of Functional Intelligent Materials,*
*National University of Singapore, 4 Science Drive 2, Singapore 117544*

Leeor Kronik

*Department of Molecular Chemistry and Materials Science,*
*Weizmann Institute of Science, Rehovoth 7610000, Israel*

Stefano Pittalis

*CNR-Istituto Nanoscienze, Via Campi 213A, I-41125 Modena, Italy*

## CONTENTS OF THE SUPPLEMENTARY MATERIAL

- Section I provides additional theoretical results;
- Section II details the orbital optimization approach used to solve EDFT problems;
- Section III details the EX22 set and optimizations and benchmarking based thereon;
- Section IV provides technical details for the other examples.

* t.gould@griffith.edu.au

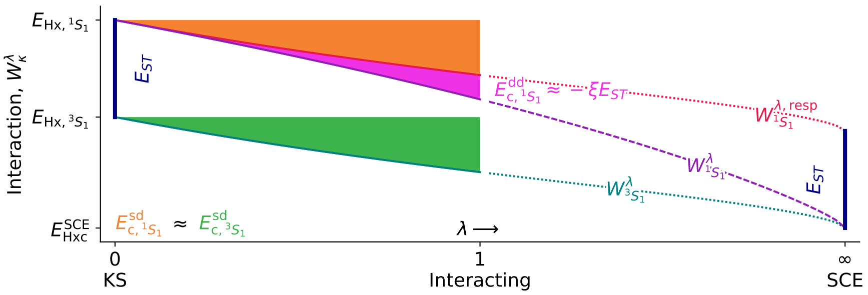


SUPPLEMENTARY FIGURE 1: Model adiabatic connection curves for the singly promoted triplet, ${}^3S_1$, and singlet, ${}^1S_1$, including exact limits. The teal dotted line and dashed purple line are $W^\lambda_{{}^3S_1}$ and $W^\lambda_{{}^1S_1}$, respectively. The red dotted line, $W^{\lambda,\mathrm{resp}}_{{}^1S_1}$, is parallel to the teal dotted line. The shaded areas are correlation energy components [see Eqs (S1) and (S2)] and are discussed in the text.

## I. ADDITIONAL THEORETICAL RESULTS

### A. A geometric illustration of the ddc model

The main text obtains a general expression for $E^{\mathrm{dd}}_{\mathrm{c},\kappa}$ by assigning different terms of an approximated integral to to the response or Coulombic part of the model. For the specific case of the triplet/singlet pair obtained by promoting one electron from the highest occupied ($\phi_h$) to the lowest unoccupied ($\phi_l$) orbital, we can use geometry and exact contraints to deduce $E^{\mathrm{dd}}_{\mathrm{c},\kappa}$, and thus provide a complementary argument that yields the same result.

Supplementary Figure 1 shows $W^\lambda_\kappa$ for a triplet ($|{}^3S_1\rangle$, teal dotted line) and singlet ($|{}^1S_1\rangle$, dashed purple line) pair evaluated at the same density. It also shows $W^{\lambda,\mathrm{resp}}_{{}^1S_1}$ (red dotted line) which the response ansatz dictates must be parallel to $W^\lambda_{{}^3S_1}$ because both states have the same density and non-interacting response. Correlation energies,

$$E_{\mathrm{c},{}^3S_1} := \int_0^1 W^\lambda_{{}^3S_1} - W^0_\kappa d\lambda = E^{\mathrm{sd}}_{\mathrm{c},{}^3S_1} \,, \tag{S1}$$

$$E^{\mathrm{sd}}_{\mathrm{c},{}^1S_1} := \int_0^1 W^{\lambda,\mathrm{resp}}_{{}^1S_1} - W^0_{{}^1S_1} d\lambda \,, \qquad E^{\mathrm{dd}}_{\mathrm{c},{}^1S_1} := \int_0^1 W^\lambda_{{}^1S_1} - W^{\lambda,\mathrm{resp}}_{{}^1S_1} d\lambda \,, \tag{S2}$$

are the shaded areas (green, orange and purple, respectively) and the parallel lines dictate that the green ($-E_{\mathrm{c},{}^3S_1}$) and orange ($-E^{\mathrm{sd}}_{\mathrm{c},{}^1S_1}$) regions have the same area.

The purple area (i.e. the integral between $W^\lambda_{{}^1S_1}$ and $W^{\lambda,\mathrm{resp}}_{{}^1S_1}$) is minus the ddc. To evaluate its area we use the recently-derived exact limits of excited electrons [1] to obtain:

$W^0_{^1S_1} = E_{\text{Hx},^1S_1} = E_{\text{Hx},^3S_1} + E_{ST} = W^0_{^3S_1} + E_{ST}$ from the Hx energy [2] of the CSFs – which are different in each case; and $W^\infty_{^1S_1} = V^{\text{SCE}}_{ee}[n_{^1S_1}] = V^{\text{SCE}}_{ee}[n_{^3S_1}] = W^\infty_{^3S_1}$ from the strictly correlated electron (SCE) energy [3] of the densities – which are the same in both cases. Geometry therefore yields,

$$E^{\text{dd}}_{\text{c},^1S_1} \propto -E_{ST} := -\xi(4[hl|lh]) = -2\xi U[\langle^1S_0|\hat{n}|^1S_1\rangle] \,, \tag{S3}$$

after recognising that $\langle^1S_0|\hat{n}|^1S_1\rangle = \sqrt{2}\phi_h\phi_l^*$ is the only relevant and non-zero transition-density for $|^1S_1\rangle$ appearing in Eq. (8) of the main text.

### B. Deeper analysis of the ddc approximation

The main text introduces the relation $W^\lambda := [1 - f_\kappa[n](\lambda)]W^0_\kappa + f_\kappa[n](\lambda)W^\infty_\kappa = [1 - f_\kappa[n](\lambda)]E_{\text{Hx},\kappa} + f_\kappa[n](\lambda)V^{\text{SCE}}_{ee}[n_\kappa]$ where $f_\kappa[n](0) = 0$, $f_\kappa[n](\lambda) = 1$, and $f_\kappa[n](\lambda)$ is monotone non-decreasing in $\lambda$. Integrating over $\lambda$ then yields $E_{\text{Hxc},\kappa} := \xi_\kappa[n]E_{\text{Hx},\kappa} + (1-\xi_\kappa[n])V^{\text{SCE}}_{ee}[n_\kappa]$ where $\xi_\kappa[n] := \int_0^1 f_\kappa[n](\lambda)d\lambda$. The level and density-dependent $\xi_\kappa[n]$ is then approximated by a single universal constant – Eq. (7) of the main text – which is later obtained empirically.

In fact, a deeper analysis of the problem reveals that the assumption that $f_\kappa[n](\lambda)$ (and thus $\xi_\kappa[n]$) is independent of $\kappa$ and $n$ is applied only at $O(\lambda^2)$. To show this result, we include the next leading order term [1] in our model to obtain,

$$f_\kappa[n_\kappa](\lambda) := (2R_\kappa[n]\lambda + K_\kappa[n]\lambda^2)b_\kappa[n](\lambda) \,. \tag{S4}$$

Here, $R_\kappa[n] := E^{\text{GL2}}_{\text{c},\kappa}/(V^{\text{SCE}}_{ee}[n_\kappa] - E_{\text{Hx},\kappa}) \geq 0$, is related to the ensemble extension [4] of Görling-Levy second-order (EGL2) perturbation theory [5]. The unitless constant $K_{\mathcal{E}}[n]$ is unknown and the function $b_\kappa[n](\lambda)$ obeys $b_\kappa[n](0) = 1$, $\partial_\lambda b_\kappa[n](0) = 0$ and $\lim_{\lambda\to\infty} \lambda^2 b_\kappa[n](\lambda) = 1$.

Integrating Eq. (S4) yields,

$$E_{\text{Hxc},\kappa} = \delta_\kappa[n]E^{\text{GL2}}_{\text{c},\kappa} + \xi'_\kappa[n]E_{\text{Hx},\kappa} + (1 - \xi'_\kappa[n])E^{\text{SCE}}_{\text{Hxc}}[n_\kappa]l; \,, \tag{S5}$$

where $\delta_\kappa[n] := 2\int_0^1 \lambda b_\kappa[n](\lambda)d\lambda$ and $\xi'_\kappa[n] := K_\kappa[n]\int_0^1 \lambda^2 b_\kappa[n](\lambda)d\lambda$. However, GL2 is a response-like theory and thus our ansatz dictates that it is part of sdc – that is, the $\delta$ term should be dealt with by $E^{\text{sd}}_{\text{xc},\kappa}$. Thus, only the terms involving $\xi'$ remain and, since these are identical in form to the original expression, we may set $\xi' \to \xi$.

## II. SOLVING THE EDFT PROBLEM THROUGH ORBITAL OPTIMIZATION

The ensemble energy of the excited state DFAs considered explicitly in the main text may all be written in general form,

$$E_{\kappa}^{\text{EDFA}} := T_s[n_\kappa] + \int n_\kappa(\boldsymbol{r})v(\boldsymbol{r})d\boldsymbol{r} + U[n_\kappa] + \sum_{P\in\text{pure}} C_P^\kappa E_{\text{xc}}^{\text{DFA}}[\rho_P] + A_\kappa(1-\xi)[hl|lh] \quad \text{(S6)}$$

where $U[n_\kappa]$ is the Hartree energy of the density. Here, $P$ indicates Slater determinant states, $|\Phi_P\rangle$ that are lowest energy in their symmetry class (gs and ts for the cases discusses in the manuscript), with reduced density matrix $\rho_P$, and corresponding particle density $n_P$. $C_P^\kappa$ are coefficients such that $\sum_P C_P^\kappa = 1$ and $\sum_P C_P^\kappa n_P = n_\kappa$. The coefficient, $A_{^1S_0} = A_{^3S_1} = 0$ for the ground and triplet states ($^1S_0$, $^3S_1$) and $A_{^1S_1} = A_{^1S_2} = 2$ for the singly- and double-excited singlets ($^1S_1$, $^1S_2$). We remind the reader that,

$$\rho_{^1S_0,\uparrow} = \rho_{^1S_0,\downarrow} = \sum_{i\leq h}\rho_i\ , \qquad \rho_{^3S_1,\uparrow} = \rho_{^1S_0,\uparrow} + \rho_l\ , \qquad \rho_{^3S_1,\downarrow} = \rho_{^1S_0,\downarrow} - \rho_h \quad \text{(S7)}$$

may be defined via $\rho_i(\boldsymbol{r},\boldsymbol{r}') \equiv \phi_i^*(\boldsymbol{r})\phi_i(\boldsymbol{r}')$.

The work also considers some special cases (doublet ground states, double excitations in cyclopentadienethione, ozone at fractional charge) where (S6) needs to be extended. These are discussed as required.

Formally, self-consistent solutions of Eq. (S6) may often be found via KS theory. However, in practice this is very difficult due to the presence of non-local exchange and (in some cases) $[hl|lh]$, so orbital solution must instead be found via ensemble generalized Kohn-Sham (EGKS) theory. [6] EGKS leads to a coupled set of equations,

$$\hat{F}_{\kappa,i}|\phi_{\kappa,i}\rangle = \epsilon_{\kappa,i}|\phi_{\kappa,i}\rangle + \sum_{j\neq i}\varepsilon_{\kappa,ij}|\phi_{\kappa,j}\rangle, \quad \text{(S8)}$$

where $\hat{F}_{\kappa,i} \equiv \hat{t} + v + \hat{v}_{\text{Hxc},\kappa,i}$ is an effective Fock operator for orbital, $i$. Here, $\hat{v}_{\text{Hxc},i}|\phi_i\rangle \equiv \frac{\delta E_{\text{Hxc}}}{f_i\delta\langle\phi_i|}$ is the effective Hxc potential for orbital $i$ with occupation $f_i^\kappa$ in state $\kappa$ with orbital energy $\epsilon_{\kappa,i}$. The terms $\varepsilon_{\kappa,ij}$ are Lagrange multipliers for orthogonality $\langle\phi_{\kappa,i}|\phi_{\kappa,j}\rangle = \delta_{ij}$. For brevity we will now drop subscripts, $\kappa$, on Fock operators, orbitals and related quantities.

Applying density functional chain rules to (S6) yields,

$$\hat{F}_i = \hat{t} + v + v_{\text{H}}[n_\kappa] + \begin{cases} \sum_P C_P^\kappa \frac{\hat{v}_{\text{xc},P\uparrow}^{\text{DFA}} + \hat{v}_{\text{xc},P\downarrow}^{\text{DFA}}}{2} & i < h\ , \\ \sum_\sigma \sum_P \frac{\theta_{h\sigma}}{f_h^\kappa} C_P^\kappa \hat{v}_{\text{xc},P\sigma}^{\text{DFA}} + \frac{2A_\kappa}{f_h^\kappa}(1-\xi)\hat{v}_{K,l}\ , & i = h\ , \\ \sum_\sigma \sum_P \frac{\theta_{l\sigma}}{f_l^\kappa} C_P^\kappa \hat{v}_{\text{xc},P\sigma}^{\text{DFA}} + \frac{2A_\kappa}{f_l^\kappa}(1-\xi)\hat{v}_{K,h}\ , & i \geq l\ . \end{cases} \quad \text{(S9)}$$

Here we used $n_\kappa = \sum_i f_i^\kappa |\phi_i|^2$ and $\rho_{P\sigma} = \sum_{i\sigma} \theta_{i\sigma}^P \rho_i$ $[\rho_i(\boldsymbol{r},\boldsymbol{r}') \equiv \phi_i^*(\boldsymbol{r})\phi_i(\boldsymbol{r}')]$; where $f_i^\kappa = \sum_P C_P^\kappa \theta_i^P$ is occupation of orbital $i$ in $n_\kappa$ and $\theta_{i\sigma}^P$ is the occupation of orbital $i$ with spin $\sigma$ in pure state $P$. The non-trivial potential terms are $\hat{v}_{\text{xc},P\sigma}^{\text{DFA}} = \frac{\delta E_{\text{xc}}^{\text{DFA}}[\tilde{\rho}_P]}{\delta \tilde{\rho}_{P\sigma}}$ (i.e. the xc potential operator from the DFA – here $\tilde{\rho}$ stands for $\rho$ or $n$ depending on the DFA) and $\hat{v}_{K,j}$ obeying $\hat{v}_{K,j}\phi_i(\boldsymbol{r}) = \phi_j(\boldsymbol{r}) \int \phi_j^*(\boldsymbol{r}')\phi_i(\boldsymbol{r}') \frac{d\boldsymbol{r}d\boldsymbol{r}'}{|\boldsymbol{r}-\boldsymbol{r}'|}$ (i.e. an exchange-like potential). For double excitations $f_h = 0$ and so $\hat{F}_h$ is ill-defined. To avoid problems we set $\hat{F}_h \equiv \hat{F}_{i<h}$.

Solving Eq. (S8) directly is numerically challenging, but a solution may be found by directly minimizing Eq. (S6) with respect to a set of orthonormal orbitals. We adopt this approach for this work, and carry out all calculations using Version 1.00 of the `Broadway` code, [7] interfaced with psi4numpy. [8, 9] `Broadway` is designed to solve a wide class of ensemble problems based on Eq. (S6) and extensions; and proceeds via the follow algorithm:

1. Begin with a typical self-consistent DFT singlet 'ground state' where all occupied orbitals are paired; and represent the resulting set (occupied and virtual) of orbitals, $\{\phi_i\}$, as a matrix, $\mathbb{C}$.

2. Use $\mathbb{C}$ to evaluate the energy, $E$, and expectation values of Fock operators, $\mathbb{F}_{ij}^k = \langle\phi_i|\hat{F}_k|\phi_j\rangle$ using the existing orbitals.

3. Unitarily transform the orbitals, $\mathbb{C} \to \exp(\mathbb{A})\mathbb{C}$, for anti-symmetric matrix $\mathbb{A}$ (discussed below) based on current orbitals and Fock operators.

4. Repeat from 2 unless the orbitals and energy are stable enough to terminate.

5. Use the final orbitals in Eq. (S6) for the final energy.

Setting the matrix $\mathbb{A}$ to have elements, $A_{ij} \propto -\langle\phi_i|f_i\hat{F}_i - f_j\hat{F}_j|\phi_j\rangle$, ensures that the energy $E_\kappa^{\text{EDFA}}$ approaches a stationary state under some assumptions about smoothness and nearness. This result may be seen by setting $\phi_i \to \phi_i + A_{ij}\phi_j$ and $\phi_j \to \phi_j - A_{ij}\phi_i$ in Eq. (S6) and evaluating the leading-order correction to the energy. `Broadway` acclerates convergence by using an approximate Hessian [10] as a pre-factor. Orbitals are therefore updated using,

$$A_{ij} = \frac{-\Delta_{ij}\Omega_{ij}}{\Omega_{ij}^2 + \eta^2}\,, \qquad \Delta_{ij} = f_i F_{ij}^i - f_j F_{ij}^j\,, \qquad \Omega_{ij} = 2|f_i - f_j||F_{ii}^i - F_{jj}^j|\,, \tag{S10}$$

where $\eta = 0.1$ regularizes (nearly-)degenerate states.

## III. EX22 BENCHMARK SET, OPTIMIZATION AND GROUND STATE BENCHMARKING

### A. EX22 benchmark set

EX22 (results and summary shown in Supplementary Table I) is composed of four subsets, two of which involve the same molecules but test a different excitation energy:

- Singlet-singlet (SS) involves excitation energies, ${}^1S_0 \to {}^1S_1$, for acrolein, butadiene, cyanoformaldehyde, cyclopentadiene, glyoxal and tetrazine;
- Triplet-singlet (TS) involves excitation energies, ${}^3S_1 \to {}^1S_1$, for the SS molecules;
- Charge-transfer (CT) involves charge-transfer excitations, ${}^1S_0 \to {}^1S_1$, for aminobenzonitrile, aniline, azulene, benzonitrile, n-phenylpyrrole and nitroaniline;
- Double excitation (DX) involves double excitation to degenerate LUMO, ${}^1S_0 \to {}^1D_2$, for BH and regular double excitations, ${}^1S_0 \to {}^1S_2$, for formaldehyde, glyoxal and nitroxyl.

It is designed to capture a diverse range of chemical and excitation physics, but be small enough to provide a reasonable norm for the unknown parameters $\xi$ and $\gamma$. The molecules in EX22 were selected on the following principles:

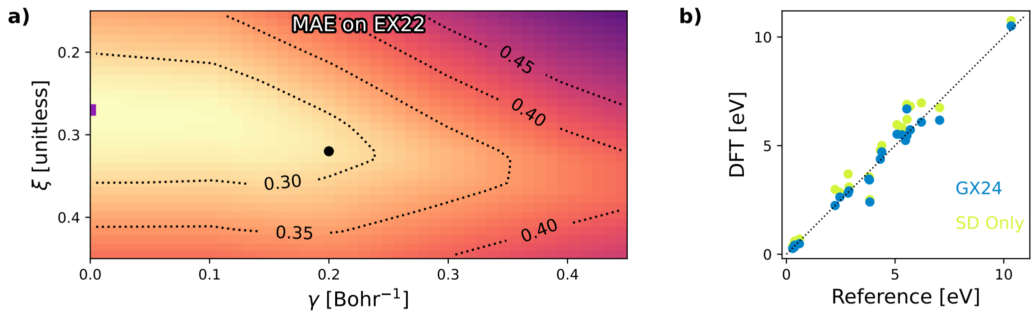


SUPPLEMENTARY FIGURE 2: **a)** Mean absolute energy values on EX22 as a function of range-separation parameter, $\gamma$, and density-driven correlation factor, $\xi$. Includes the true optimal value (red square at the far left) and selected value with $\gamma = 0.2$ and $\xi = 0.32$ (black dot). **b)** Energies for EX22 predicted using GX24 (blue dots) and the state-driven only (lime dots) part of GX24 (i.e. using $\xi = 0$). Black dotted line indicates perfect agreement.

- Minimize molecules with high symmetry, to ensure the norming was not biased by symmetries;
- Ensure that all single excitations covered diverse chemistry:
  - mix of double bonds: acrolein, butadiene, glyoxal, cyclopentadiene; and triple bonds: cyanoformaldehyde;
  - cyclic: cyclopentadiene, tetrazine; and bicyclic: n-phenylpyrrole;
  - aromaticity: tetrazine, benzonitrile, aminobenzonitrile, aniline, azulene, nitroaniline;
  - all carbon: azulene, butadiene, cyclopentadiene; some with nitrogen; some with oxygen (with some overlap with nitrogen)
- Acrolein, butadiene and glyoxal share the same structural motif with 1, 0 and 2 aldehyde groups respectively and the combination of similarities and differences have made them attractive systems to study previously; [11–13]
- Azulene violates Kasha's rule with emission from ${}^1S_2 \to {}^1S_0$.

### B. Key results from EX22

Supplementary Figure 2 (left) shows mean absolute errors for GX24 evaluated with a range of $\gamma$ and $\xi$ values. The true optimal value (indicated by a red square at the far left) is for $\gamma = 0$ (i.e. no range-separation) and $\xi = 0.27$ and yields a mean absolute error (MAE) of 0.29 eV. Setting $\gamma = 0.2$ and $\xi = 0.32$ (indicated by a black dot) increases the MAE to 0.31 eV but has correct charge transfer physics and is therefore used in GX24.

*Technical notes*

The double excitation in BH is to a degenerate LUMO and we thus need to adapt Eq. (S6). The resulting energy expression,

$$E^{\text{EDFA}}_{\text{BH-dx}} := T_s[n_\kappa] + \int n_\kappa(\boldsymbol{r})v(\boldsymbol{r})d\boldsymbol{r} + E_{\text{H}}[n_\kappa] + E^{\text{DFA}}_{\text{xc,ts}_1} + E^{\text{DFA}}_{\text{xc,ts}_2} - E^{\text{DFA}}_{\text{xc,gs}} + (1-\xi)[hl_1|l_1h] + (1-\xi)[hl_2|l_2h] + (1-\xi)[l_1l_2|l_2l_1] \tag{S11}$$

is like an average over triplet states ($ts_1$ and $ts_2$) involving the degenerate LUMOs ($l_1$ and $l_2$); and also includes an extra term for interactions between the two LUMOs. The minimum may then be found using `Broadway`.

To norm GX24 we computed variational minima of Eq. (S6) and (S11) in a grid of values, $\gamma_j$ and $\xi_j$, to obtain $\Delta E_X(\gamma_i, \xi_j, )$ for all 22 excitations (subscript $X$) in EX22. We varied $\gamma_i$ from zero to 0.5 in steps of 0.1 and $\xi_j$ from zero to 0.5 in steps of 0.05. To accelerate calculations and avoid local minima we seeded each new $\xi_{j+1}$ (at fixed $\gamma_i$) by using the converged orbitals from the previous $\xi_j$, instead of the ground state. The energies of each excitation varied quite slowly with $\gamma_i$ and $\xi_j$, so we obtainen $\Delta E_X(\gamma, \xi, )$ at arbitrary $\gamma$ and $\xi$ via linearly interpolation of nearby known values. We then used the interpolated values to calculate mean absolute errors, $\text{MAE}(\xi, \gamma) = \frac{1}{22} \sum_X |\Delta E_X(\xi, \gamma) - \Delta E_X^{\text{ref}}|$, to produce the results in Supplementary Figure 2 and so obtain optimal values of $\xi$ at fixed $\gamma$. Results in Supplementary Tables I and III are recomputed using $\gamma = 0.2$ and $\xi = 0.32$.

SUPPLEMENTARY TABLE I: Excitation energies computed using the DFA from the present work compared to benchmark values from QuestDB [11–13] plus BH [14]

| Name | Key | Error | GX24 | Ref. |
|---|---|---|---|---|
| | | Singlet-singlet | | |
| acrolein | SS1 | -0.33 | 3.46 | 3.79 |
| butadiene | SS2 | -0.13 | 6.08 | 6.21 |
| cyanoformaldehyde | SS3 | -0.40 | 3.42 | 3.82 |
| cyclopentadiene | SS4 | -0.08 | 5.47 | 5.55 |
| glyoxal | SS5 | 0.04 | 2.92 | 2.88 |
| tetrazine | SS6 | 0.17 | 2.63 | 2.46 |
| MAE(SS) | | 0.19 | | |
| MAPE(SS) | | 5.16 | | |
| | | Triplet-singlet | | |
| acrolein | ST1 | -0.02 | 0.27 | 0.29 |
| butadiene | ST2 | -0.03 | 2.81 | 2.84 |
| cyanoformaldehyde | ST3 | -0.04 | 0.33 | 0.37 |
| cyclopentadiene | ST4 | 0.00 | 2.24 | 2.24 |
| glyoxal | ST5 | 0.04 | 0.42 | 0.38 |
| tetrazine | ST6 | -0.11 | 0.49 | 0.60 |
| MAE(ST) | | 0.04 | | |
| MAPE(ST) | | 8.34 | | |
| | | All EX22 | | |
| ME | | -0.05 | | |
| MAE | | 0.29 | | |
| RMSD | | 0.47 | | |
| MPE | | -2.5% | | |
| MAPE | | 8.1% | | |
| Kendall tau | | 0.87 | | |

SUPPLEMENTARY TABLE II: Continuation of Table I.

| Name | Key | Error | GX24 | Ref. |
|---|---|---|---|---|
| | | Charge transfer | | |
| aminobenzonitrile | CT1 | 0.43 | 5.52 | 5.09 |
| aniline | CT2 | -0.24 | 5.24 | 5.48 |
| azulene | CT3 | -1.43 | 2.41 | 3.84 |
| benzonitrile | CT4 | -0.88 | 6.17 | 7.05 |
| n-phenylpyrrole | CT5 | 0.18 | 5.50 | 5.32 |
| nitroaniline | CT6 | 0.32 | 4.71 | 4.39 |
| MAE(CT) | | 0.58 | | |
| MAPE(CT) | | 12.23 | | |
| | | Double excitation | | |
| BH | DX1 | 0.03 | 5.73 | 5.70 |
| formaldehyde | DX2 | 0.17 | 10.51 | 10.34 |
| glyoxal | DX3 | 1.15 | 6.69 | 5.54 |
| nitroxyl | DX4 | 0.06 | 4.38 | 4.32 |
| MAE(DX) | | 0.35 | | |
| MAPE(DX) | | 6.03 | | |
| | | All EX22 | | |
| ME | | -0.05 | | |
| MAE | | 0.29 | | |
| RMSD | | 0.47 | | |
| MPE | | -2.5% | | |
| MAPE | | 8.1% | | |
| Kendall tau | | 0.87 | | |

| | SS1 | SS2 | SS3 | SS4 | SS5 | SS6 | MAE |
|---|---|---|---|---|---|---|---|
| Ref. | 3.79 | 6.21 | 3.82 | 5.55 | 2.88 | 2.46 | 4.12 |
| GX24 | -0.33 | -0.13 | -0.40 | -0.08 | 0.04 | 0.17 | 0.19 |
| SD only | -0.23 | 0.75 | -0.27 | 0.66 | 0.22 | 0.39 | 0.42 |
| | ST1 | ST2 | ST3 | ST4 | ST5 | ST6 | MAE |
| Ref. | 0.29 | 2.84 | 0.37 | 2.24 | 0.38 | 0.60 | 1.12 |
| GX24 | -0.02 | -0.03 | -0.04 | 0.00 | 0.04 | -0.11 | 0.04 |
| SD only | 0.08 | 0.85 | 0.09 | 0.74 | 0.22 | 0.10 | 0.35 |
| | CT1 | CT2 | CT3 | CT4 | CT5 | CT6 | MAE |
| Ref. | 5.09 | 5.48 | 3.84 | 7.05 | 5.32 | 4.39 | 5.20 |
| GX24 | 0.43 | -0.24 | -1.43 | -0.88 | 0.18 | 0.32 | 0.58 |
| SD only | 0.87 | 0.05 | -1.33 | -0.30 | 0.52 | 0.61 | 0.61 |
| | DX1 | DX2 | DX3 | DX4 | MAE | | |
| Ref. | 5.70 | 10.34 | 5.54 | 4.32 | 6.47 | | |
| GX24 | 0.03 | 0.17 | 1.15 | 0.06 | 0.35 | | |
| SD only | 1.11 | 0.42 | 1.36 | 0.47 | 0.84 | | |

SUPPLEMENTARY TABLE III: Summary of errors (in eV) in GX24 and GX24 with only the state-driven term, i.e. with no density-driven EDFA. The overall MAE are 0.29 eV and that of the SD only part is 0.53 eV.

### C. Ground state benchmarking with the poison set P30-10

SUPPLEMENTARY TABLE IV: Mean absolute errors [eV] and mean absolute percent errors over P30-10 of selected functional, and the ensemble DFA of the main text.

| Error | PBE0 | B3LYP | CAM-B3LYP | $\omega$B97X-V | GX24 |
|---|---|---|---|---|---|
| Mean absolute error | 0.60 | 0.69 | 0.63 | 0.50 | 0.65 |
| Mean absolute % error | 48% | 58% | 43% | 33% | 23% |

Before proceeding to excited states, we do a sanity check by testing the performance of GX24 on ground states. While the ultimate goal of GX24 is excited state prediction, its performance on ground states does matter because we are usually interested in the excitation gap, i.e. the difference between an excited state energy and its ground state counterpart.

Specifically, we test GX24 on the P30-10 benchmark set of molecules with up to 10 atoms, to test its ability to capture difficult ground state problems that we expect have similar chemical physics to difficult excited state problems. Large scale benchmarking of DFAs has become a popular pastime, using benchmark sets of 1000s of reactions. However, such large benchmarking is sub-optimal in some ways. Firstly, there is a large amount of redundant infromation in large benchmark sets, with subsets of just 50 almost able to reproduce statistics for full sets. [15]. The huge redundancy also masks failure cases, by

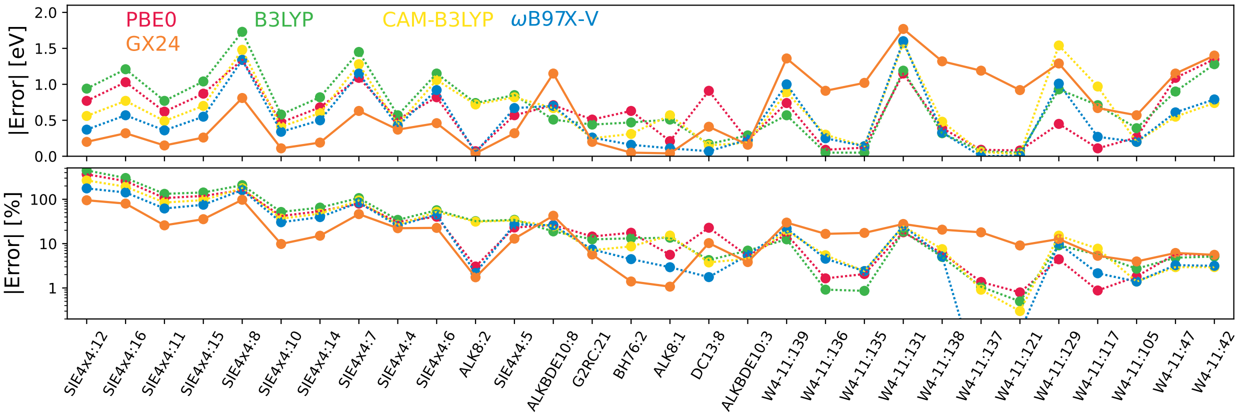


SUPPLEMENTARY FIGURE 3: Absolute errors (top panel) and percent absolute errors (bottom panel) for the thirty processes in P30-10, using a variety of different DFAs. Molecules are ordered by their reaction energy.

reducing their impact on statistics. To overcome these limitations, the poison sets of difficult benchmark problems [16] were designed to carefully scrutinize failures of DFAs on tough problems.

Results for the thirty processes of P30-10 are provided in Supplementary Figure 3. We use the cc-pvtz basis set to match the EX22 benchmarking. Supplementary Table IV provides key statistics to reveal that GX24 (with no empirical parameters trained on ground states) is the second worse performer on mean absolute errors, with only B3LYP (three empricial parameters) doing worse. However, on mean absolute % errors it is the top performer, beating even $\omega$B97X-V, which is an exceptional empirical ground state functional with ten empirical parameters optimized on ground states. Thus, while GX24 is unlikely to become a 'first choice' for ground states, its performance is sufficiently reliable that it is unlikely to hamper predictions.

*Technical notes*

Note, Eq. (S6) is only valid for ground or triplet states with an even number of paired electrons, whereas P30-10 contains ground states involving odd electron number. To address these cases we adapt the results for excited states to obtain,

$$\hat{F}_{i\in\text{docc}} = \tfrac{1}{2}(\hat{F}^{\uparrow}_{\text{UKS}} + \hat{F}^{\downarrow}_{\text{UKS}}) , \qquad \hat{F}_{i\in\text{socc}} = \hat{F}^{\uparrow}_{\text{UKS}} , \tag{S12}$$

as the effective Fock operators for the double occupied (docc) and singly occupied (socc) orbitals, where $\hat{F}^{\sigma}$ indicates the $\sigma$ Fock orbital from unrestricted Kohn-Sham theory, using GX24 as the DFA. The minimum may then be found using `Broadway`.

## IV. RESULTS AND TECHNICAL DETAILS FOR EXAMPLES

### A. 'Easy' and 'Hard' low-lying excited states

Additional excited state results, including TDA and full TDDFT values are provided in Supplementary Tables V and VI. GX24 results were computed using the method of Supplementary Section II. TDA and TDDFT results were computed for this work, using pyscf. [17] Basis sets are the same for EDFT and TDDFT and detailed in the table captions.

Table V shows relatively 'easy' excitations, in the sense that they involve well-defined orbitals and transitions that do not pose a fundamental challenge for TDDFT. However, the nature of these excitations (Rydberg and charge transfer) exposes limitations of DFT as they require long-range corrections (as in CAM-B3LYP or GX24) to capture correct qualitative behaviour. They therefore offer an effective quantitative test of GX24 and CAM-B3LYP on non-trivial excitations.

The systems shown in Table VI are all very challenging for currently available TDDFT approximations, due to known fundamental failures with double excitations. They therefore test the effectiveness of GX24 for excitations that are nearly impossible for TDDFAs. The test set includes all excitations from Ref. 18 with energies less than 5 eV except: i) nitroxyl, as it is part of EX22; and ii) $C_2$ and $C_3$ as both require sophisticated treatment to deal with their rotational symmetries. Only three of the excitations (the two in Criegee's intermediate and one in octatetraene) can be captured *at all* in adiabatic approximations to TDDFT, so relevant statistics cover these three cases only.

*Technical notes*

Some molecules needed special treatment. 1) The Criegee's intermediates were computed using the natural orbitals of an unrestriced Kohn-Sham triplet state as a starting point, as a singlet starting point became trapped in a local minima. 2) Cyclopentadienethione has a double excitation to $|1^2\ldots(h-2)^2(h-1)hl^2\rangle$ that involves double promotion from two occupied orbitals to one virtual orbital. It is handled similarly to the case of BH, via,

$$E_{\rm Hxc,cycp} = E_{\rm H,dx} + E^{\rm DFA}_{\rm xc,ts_1} + E^{\rm DFA}_{\rm xc,ts_2} - E^{\rm DFA}_{\rm xc,gs} + \tfrac{1}{2}(E'_{ST,(h-1)l} + E'_{ST,hl}) + E'_{ST,(h-1)h}\,. \tag{S13}$$

SUPPLEMENTARY TABLE V: Rydberg excitations in water, $H_2S$ and ammonia, and charge-transfer in HCl. All calculated with aug-cc-pvtz basis set. Note, TDDFT predicts some lower energy excitations but we restrict to values closest to TDA. MAE = mean absoute error, RMSD = root mean square deviation, Max = maximum absolute error.

| $\Delta E$ [eV] | | Water | | $H_2S$ | | Ammonia | | HCl | MAE | RMSD | Max |
|---|---|---|---|---|---|---|---|---|---|---|---|
| TBE | 7.70 | 9.47 | 9.97 | 6.10 | 6.29 | 6.66 | 8.21 | 7.86 | | | |
| GX24 | 7.42 | 9.11 | 9.71 | 6.09 | 6.32 | 6.50 | 7.97 | 7.79 | | | |
| Err | -0.28 | -0.36 | -0.26 | -0.01 | 0.03 | -0.16 | -0.24 | -0.07 | 0.18 | 0.21 | 0.36 |
| TDA | 6.74 | 7.14 | 8.56 | 5.52 | 5.60 | 5.91 | 6.21 | 6.99 | | | |
| Err | -0.96 | -2.33 | -1.41 | -0.58 | -0.69 | -0.75 | -2.00 | -0.87 | 1.20 | 1.34 | 2.33 |
| TDDFT | 6.72 | 7.13 | 8.54 | 5.45 | 5.57 | 5.89 | 6.20 | 6.95 | | | |
| Err | -0.98 | -2.34 | -1.43 | -0.65 | -0.72 | -0.77 | -2.01 | -0.91 | 1.23 | 1.36 | 2.34 |

Subscripts gs, $ts_{1,2}$ and dx indicate densities: $n_{\text{gs}} = 2\sum_{i=0}^{h} n_i$, $n_{\text{ts}_1} = 2\sum_{i=0}^{h-2} n_i + n_{h-1} + 2n_h + n_l$, $n_{\text{ts}_2} = 2\sum_{i=0}^{h-2} n_i + 2n_{h-1} + n_h + n_l$ and $n_{\text{dx}} = 2\sum_{i=0}^{h-2} n_i + n_{h-1} + n_h + 2n_l$; and $E'_{ST,ft} := 2(1-\xi)[ft|tf]$. These special cases can all be addressed by `Broadway`.

SUPPLEMENTARY TABLE VI: Double excitation energies (cycp, cycc, borole, nme, tetrazine) or excitations with strong double characteristics (Criegee's, oct). All calculated with cc-pvtz basis set, except Criegee's calculated with aug-cc-pvtz. [a]

| $\Delta E$ [eV] | Criegee's | | cycp | cycb | oct | borole | nme | tetrazine | MAE | RMSD | Max |
|---|---|---|---|---|---|---|---|---|---|---|---|
| TBE | 2.40 | 3.72 | 3.16 | 4.04 | 4.68 | 4.71 | 4.73 | 4.95 | | | |
| GX24 | 1.74 | 2.93 | 3.03 | 4.52 | 4.43 | 5.40 | 4.81 | 5.91 | | | |
| Err | -0.66 | -0.79 | -0.13 | 0.48 | -0.25 | 0.69 | 0.08 | 0.96 | 0.50 | 0.59 | 0.96 |
| TDA | 0.09 | 0.34 | – | – | 2.18 | – | – | – | | | |
| Err | -2.31 | -3.38 | – | – | -2.50 | – | – | – | 2.73 | 2.77 | 3.38 |
| TDDFT | 0.87 | 0.92 | – | – | 1.49 | – | – | – | | | |
| Err | -1.53 | -2.80 | – | – | -3.19 | – | – | – | 2.51 | 2.60 | 3.19 |

[a] cycp=cyclopentadienethione, cycb=cyclobutadiene, oct=octatetraene, nme=nitrosomethane

### B. Electron affinity calculations

Evaluating the electron affinity at fractional charge involves extending the previous results to charged excitations. The interacting density and energy of fractional charges are linear interpolations between neutral (e.g. $O_3$) and charged (e.g. $O_3^-$) systems; and the exact H and x energy *expressions* are also linear in charge. [19, 20] After making the usual assumption that state-driven correlations obey the same combination laws as exchange, the relevant terms for a singlet neutral system are,

$$\rho_\uparrow^q = \sum_{i\leq h} \rho_i^q + q\rho_l^q \ , \qquad \rho_\downarrow^q = \sum_{i\leq h} \rho_i^q \ , \tag{S14}$$

$$\mathcal{E}_{\rm H}^q = (1-q)E_{\rm H}[n^{0@q}] + qE_{\rm H}[n^{1@q}] = U[n^q] + q(1-q)U[n_l^q] \ , \tag{S15}$$

$$\mathcal{E}_{\rm xc}^{{\rm sd},q} = (1-q)E_{\rm xc}^{\rm GX24}[\rho^{0@q}] + qE_{\rm xc}^{\rm GX24}[\rho^{1@q}] \tag{S16}$$

$$\mathcal{E}_{\rm c}^{{\rm dd},q} = \xi\big\{U[n^q] - \mathcal{E}_{\rm H}^q\big\} = -\xi q(1-q)U[n_l^q] = -\tfrac{1}{2}\xi q(1-q)[ll|ll] \ , \tag{S17}$$

where $q$ is the number of excess electrons that serves to define the ensemble, $h$ is the HOMO of the neutral system and $l$ is the LUMO that captures the excess electron. Although (S15) and (S16) are *prima facie* linear in $q$, they are not truly linear because the self-consistent Kohn-Sham orbitals, $\phi_i^q$, vary with $q$ and thus the 1RDMs $[\rho_i^q(\boldsymbol{r},\boldsymbol{r}') = \phi_i^{*q}(\boldsymbol{r})\phi_i^q(\boldsymbol{r}')]$ and densities $[n_i^q(\boldsymbol{r}) = |\phi_i^q(\boldsymbol{r})^2]$ depend on $q$ – as indicated by superscripts on $\phi$, $\rho$ and $n$ terms. The notation $\rho^{q'@q}$ indicates a 1RDM for charge $q'$ using orbitals from charge $q$, so that $\rho_\uparrow^{q'@q} = \sum_{i\leq h}\rho_i^q + q'\rho_l^q$ and $\rho_\downarrow^{q'@Q} = \sum_{i\leq h}\rho_i^q$. Similar reasoning yields (S17) also for a doublet neutral system.

Notably, the DD correlation energy expression (S17) – obtained directly from $\xi(U[n] - \mathcal{E}_{\rm H}[n])$ and (S15) – depends on a Hartree-like integral, instead of the exchange-like integrals found in neutral excitations. Thus, it represents a physically (charged versus neutral) and mathematically (Hartree-like versus exchange-like) different model of DD correlations that is obtained from the same underlying principles as the neutral case already considered.

Calculations are carried out with the aug-cc-pvtz basis set using `Broadway`. Ignoring DD correlations (i.e. setting $\xi = 0$) leads to substantial non-linearities in the energy, caused by Kohn-Sham orbital relaxation. Including Eq. (S17) cancels out most of the non-linearity and restore qualitative and quantitative agreement with experiment.

[1] T. Gould, D. P. Kooi, P. Gori-Giorgi, and S. Pittalis, Electronic excited states in extreme limits via ensemble density functionals, Phys. Rev. Lett. **130**, 106401 (2023).

[2] T. Gould and S. Pittalis, Hartree and exchange in ensemble density functional theory: Avoiding the nonuniqueness disaster, Phys. Rev. Lett. **119**, 243001 (2017).

[3] M. Seidl, J. P. Perdew, and M. Levy, Strictly correlated electrons in density-functional theory, Phys. Rev. A **59**, 51 (1999).

[4] Z. Yang, Second-order perturbative correlation energy functional in the ensemble density-functional theory, Phys. Rev. A **104**, 052806 (2021).

[5] A. Görling and M. Levy, Correlation-energy functional and its high-density limit obtained from a coupling-constant perturbation expansion, Phys. Rev. B **47**, 13105 (1993).

[6] T. Gould and L. Kronik, Ensemble generalized Kohn-Sham theory: The good, the bad, and the ugly, J. Chem. Phys. **154**, 094125 (2021).

[7] T. Gould, Broadway - an EDFT library for python (2024).

[8] R. M. Parrish, L. A. Burns, D. G. A. Smith, A. C. Simmonett, A. E. DePrince, E. G. Hohenstein, U. Bozkaya, A. Y. Sokolov, R. D. Remigio, R. M. Richard, J. F. Gonthier, A. M. James, H. R. McAlexander, A. Kumar, M. Saitow, X. Wang, B. P. Pritchard, P. Verma, H. F. Schaefer, K. Patkowski, R. A. King, E. F. Valeev, F. A. Evangelista, J. M. Turney, T. D. Crawford, and C. D. Sherrill, Psi4 1.1: An open-source electronic structure program emphasizing automation, advanced libraries, and interoperability, J. Chem. Theory Comput. **13**, 3185 (2017).

[9] D. G. A. Smith, L. A. Burns, D. A. Sirianni, D. R. Nascimento, A. Kumar, A. M. James, J. B. Schriber, T. Zhang, B. Zhang, A. S. Abbott, E. J. Berquist, M. H. Lechner, L. A. Cunha, A. G. Heide, J. M. Waldrop, T. Y. Takeshita, A. Alenaizan, D. Neuhauser, R. A. King, A. C. Simmonett, J. M. Turney, H. F. Schaefer, F. A. Evangelista, A. E. DePrince, T. D. Crawford, K. Patkowski, and C. D. Sherrill, Psi4numpy: An interactive quantum chemistry programming environment for reference implementations and rapid development, J. Chem. Theory Comput. **14**, 3504 (2018).

[10] G. Levi, A. V. Ivanov, and H. Jónsson, Variational calculations of excited states via direct optimization of the orbitals in dft, Faraday Discuss. **224**, 448 (2020).

[11] P.-F. Loos, A. Scemama, A. Blondel, Y. Garniron, M. Caffarel, and D. Jacquemin, A mountaineering strategy to excited states: Highly accurate reference energies and benchmarks, J. Chem. Theory Comput. **14**, 4360 (2018).

[12] P.-F. Loos, N. Galland, and D. Jacquemin, Theoretical 0-0 energies with chemical accuracy, J. Phys. Chem. Lett. **9**, 4646 (2018).

[13] P.-F. Loos, M. Boggio-Pasqua, A. Scemama, M. Caffarel, and D. Jacquemin, Reference energies for double excitations, J. Chem. Theory Comput. **15**, 1939 (2019).

[14] T. Gould, L. Kronik, and S. Pittalis, Double excitations in molecules from ensemble density functionals: Theory and approximations, Phys. Rev. A **104**, 022803 (2021).

[15] T. Gould, 'diet gmtkn55'offers accelerated benchmarking through a representative subset approach, Phys. Chem. Chem. Phys. **20**, 27735 (2018).

[16] T. Gould and S. G. Dale, Poisoning density functional theory with benchmark sets of difficult systems, Phys. Chem. Chem. Phys. **24**, 6398 (2022).

[17] Q. Sun, X. Zhang, S. Banerjee, P. Bao, M. Barbry, N. S. Blunt, N. A. Bogdanov, G. H. Booth, J. Chen, Z.-H. Cui, J. J. Eriksen, Y. Gao, S. Guo, J. Hermann, M. R. Hermes, K. Koh, P. Koval, S. Lehtola, Z. Li, J. Liu, N. Mardirossian, J. D. McClain, M. Motta, B. Mussard, H. Q. Pham, A. Pulkin, W. Purwanto, P. J. Robinson, E. Ronca, E. R. Sayfutyarova, M. Scheurer, H. F. Schurkus, J. E. T. Smith, C. Sun, S.-N. Sun, S. Upadhyay, L. K. Wagner, X. Wang, A. White, J. D. Whitfield, M. J. Williamson, S. Wouters, J. Yang, J. M. Yu, T. Zhu, T. C. Berkelbach, S. Sharma, A. Y. Sokolov, and G. K.-L. Chan, Recent developments in the pyscf program package, J. Chem. Phys. **153**, 10.1063/5.0006074 (2020).

[18] F. Kossoski, M. Boggio-Pasqua, P.-F. Loos, and D. Jacquemin, Reference energies for double excitations: Improvement and extension, J. Chem. Theory Comput. 10.1021/acs.jctc.4c00410 (2024).

[19] T. Gould and J. F. Dobson, The flexible nature of exchange, correlation, and Hartree physics: Resolving "delocalization" errors in a "correlation free" density functional, J. Chem. Phys. **138**, 014103 (2013).

[20] T. Gould, G. Stefanucci, and S. Pittalis, Ensemble density functional theory: Insight from the fluctuation-dissipation theorem, Phys. Rev. Lett. **125**, 233001 (2020).
